# Supplementary material for: Nonlinear Rheology in a Model Biological Tissue
Source: arXiv:1611.05282 ancillary file (2017-04-17)
Supplement: Supplementary file 1 [file supplmat-final.pdf]

# – Supplemental material –
# Nonlinear Rheology in a Model Biological Tissue

D. A. Matoz-Fernandez,[1,*] Elisabeth Agoritsas,[1,2,†] Jean-Louis Barrat,[1] Eric Bertin,[1] and Kirsten Martens[1]

[1] *Université Grenoble Alpes & CNRS, LIPHY, F-38000 Grenoble, France*

[2] *Laboratoire de Physique Théorique, ENS & PSL University, UPMC & Sorbonne Universités, F-75005 Paris, France*

## HYBRID STOCHASTIC PROCESS

One underlying interpretation of the Hébraud-Lequeux (HL) model [1] and its generalisations [2, 3] is a hybrid stochastic process for the local shear stress $\sigma_i(t)$ and the local yield stress $\sigma_{c,i}(t)$, with $i$ indexing the position of the mesoscopic box on which the local shear is defined. In a simplified mean-field picture, this stochastic process is assumed to be modelled by a combined Langevin and resetting dynamics of the scalar shear stress. First, the Langevin dynamics is given by

$$\partial_t \sigma(t) = G_0 \dot{\gamma} + \xi_{\text{mec}}(t) \qquad \text{(S1)}$$

with $G_0$ the average local elastic modulus, and $\dot{\gamma}$ the external shear rate (assumed to be constant). In other words, the local stress $\sigma(t)$ fluctuates diffusively around its external elastic loading $G_0\dot{\gamma}t$, according to a Gaussian noise $\xi_{\text{mec}}(t)$ fully determined by:

$$\begin{cases} \langle \xi_{\text{mec}}(t) \rangle = 0 \\ \langle \xi_{\text{mec}}(t) \xi_{\text{mec}}(t') \rangle = 2D(t)\delta(t-t') \end{cases} \qquad \text{(S2)}$$

Secondly, the resetting dynamics is defined as follows. Once the local stress $\sigma(t)$ exceeds the local yield stress $\sigma_c(t)$, it might trigger a local plastic event at a fixed plastic rate $1/\tau$, which would in turn fully relax the local stress, and then refresh the local yield stress by picking a random value according to the *a priori* distribution $\rho(\sigma_c')$. Thirdly, the elastic redistribution of stress to the neighbouring sites is taken into account via a coupling of the amplitude $\propto \sqrt{D(t)}$ of the mechanical noise $\xi_{\text{mec}}(t)$ to the global plastic activity $\Gamma(t) = \left\langle \frac{1}{\tau}\theta(|\sigma| - \sigma_c) \right\rangle$.

The novelty here is that we allow for two distinct contributions to the mechanical noise, on the one hand $\xi_{\text{pl}}(t)$ which stems from the sum of simultaneous plastic events throughout the system, and on the other hand $\xi_{\text{act}}(t)$ which stems for instance from the internal activity, as apoptosis and cell division in a biological tissue, or from an external shaking of the system, as in experiments on dense granular materials [4]. Assuming that both those noises are Gaussian, that they are independent translates, and that we can neglect the correlation in time (*i.e.* that the plastic events are almost simultaneous):

$$\xi_{\text{mec}}(t) = \xi_{\text{pl}}(t) + \xi_{\text{act}}(t), \quad \langle \xi_{\text{pl}}(t) \xi_{\text{act}}(t) \rangle = 0 \qquad \text{(S3)}$$

$$\begin{cases} \langle \xi_{\text{pl}}(t) \rangle = 0 \\ \langle \xi_{\text{pl}}(t) \xi_{\text{pl}}(t') \rangle = 2\alpha\Gamma(t)\delta(t-t') \end{cases} \qquad \text{(S4)}$$

$$\begin{cases} \langle \xi_{\text{act}}(t) \rangle = 0 \\ \langle \xi_{\text{act}}(t) \xi_{\text{act}}(t') \rangle = 2D_0\delta(t-t') \end{cases} \qquad \text{(S5)}$$

encoding the coupling between the mechanical noise and the plastic activity in the following closure relation:

$$D(t) = \alpha\,\Gamma(t) + D_0 \qquad \text{(S6)}$$

and the following evolution equation for the probability distribution (PDF) of local stress $\sigma$ and local yield stress $\sigma_c$ at a time $t$:

$$\begin{aligned} \partial_t \mathcal{P}(\sigma, \sigma_c, t) = &- G_0 \dot{\gamma}\, \partial_\sigma \mathcal{P} + D(t)\, \partial_\sigma^2 \mathcal{P} \\ &- \frac{1}{\tau} \theta(|\sigma| - \sigma_c)\, \mathcal{P} + \Gamma(t)\, \rho(\sigma_c)\, \delta(\sigma) \end{aligned} \qquad \text{(S7)}$$

$$\Gamma(t) = \frac{1}{\tau} \int_0^\infty d\sigma_c \int_{|\sigma| > \sigma_c} d\sigma\, \mathcal{P}(\sigma, \sigma_c, t) \qquad \text{(S8)}$$

The steady state at constant shear rate and $D_0 = 0$ has been studied in Ref. [2] for a generic distribution $\rho(\sigma_c)$, and previously with respect to the original HL model. Its generalisations with a partial relaxation of stress after a local plastic event are discussed for instance in Ref. [3], in the broader framework of athermal local-yield stress (ALYS) models.

## STEADY-STATE SOLUTION AT FIXED $\dot{\gamma}$

We consider the steady-state solution of the original HL model, adapting the expressions for the disordered HL model given in Ref. [2] by assuming a single value for the local yield stress $\sigma_c$ (*i.e.* $\rho(\sigma_c') = \delta(\sigma_c' - \sigma_c)$).

### At fixed diffusion coefficient $D$

We first recall the expressions at fixed diffusion coefficient $D$ for the global plastic activity $\Gamma = \Gamma(D, \dot{\gamma})$ and the mean stress $\sigma_M = \sigma_M(D, \dot{\gamma})$:

$$\Gamma\tau = \frac{D\tau}{\tilde{f}_{\sigma_c}\left(\sqrt{D\tau}, \frac{G_0\dot{\gamma}\tau}{D\tau}\right)} \qquad \text{(S9)}$$

where the structure of the explicit dependence suggests to define the following variables with $x = \sqrt{D\tau}$ and $y = G_0\dot{\gamma}\tau/x^2$, and

$$\tilde{f}_{\sigma_c}(x,y) - x^2 = \frac{\sigma_c}{y} \frac{1 + \left(\sqrt{1+\frac{4}{x^2y^2}} + \frac{2}{\sigma_c y}\right)\tanh\left(\frac{\sigma_c y}{2}\right)}{\tanh\left(\frac{\sigma_c y}{2}\right) + \sqrt{1+\frac{4}{x^2y^2}}} \quad \text{(S10)}$$

These last two equations correspond respectively to Eqs. (10) and (14) of Ref. [2].

As for the mean stress, we distinguish the contributions of the overstressed sites ($|\sigma| > \sigma_c$) and of the understressed sites ($|\sigma| < \sigma_c$), adapting Eqs. (C7), (C8) and (C9) of Ref. [2] at fixed $\sigma_c$:

$$\sigma_M^{(\text{over})} = G_0\dot{\gamma}\tau \quad \text{(S11)}$$

$$\sigma_M^{(\text{under})} = \frac{1}{y}\left[\frac{\sigma_c^2/2 - \tilde{f}_{\sigma_c}(x,y) + x^2}{\tilde{f}_{\sigma_c}(x,y)}\right] + \frac{1}{y^2\,\tilde{f}_{\sigma_c}(x,y)} \frac{2\sigma_c}{\sqrt{1+\frac{4}{x^2y^2}} + \tanh\left(\frac{\sigma_c y}{2}\right)} \quad \text{(S12)}$$

$$\sigma_M = \sigma_M^{(\text{over})} + \sigma_M^{(\text{under})} \quad \text{(S13)}$$

Together, the last four expressions allow to compute the mean stress as a function of the following parameters $\{G_0, \dot{\gamma}, \tau, \sigma_c, D\}$, or more precisely $\{G_0\dot{\gamma}\tau, \sigma_c, \sqrt{D\tau}\}$.

### Solving the modified closure relation at $D_0 > 0$

The nonlinear physics in the HL predicted flow curve arises because of the coupling between the plastic activity and the fluctuations of local stress, quantified by the diffusion coefficient. In the original HL model, this coupling was assumed to be linear; here we assume more generally that it is affine with a finite diffusion coefficient threshold $D_0 > 0$. In other words, we start from the closure relation:

$$D = \alpha\,\Gamma(D) + D_0 \quad \text{(S14)}$$

$$\iff \alpha\frac{D}{D - D_0} \overset{\text{(S10)}}{=} \tilde{f}_{\sigma_c}\left(\sqrt{D\tau}, \frac{G_0\dot{\gamma}\tau}{D\tau}\right) \quad \text{(S15)}$$

This equation has unfortunately no explicit analytical solution that would yield $D = D(G_0\dot{\gamma}\tau, \sigma_c, \alpha, \sqrt{D_0\tau})$. Nevertheless, the diffusion coefficient can be geometrically determined by the intersection of $\tilde{f}_{\sigma_c}\left(\sqrt{D\tau}, \frac{G_0\dot{\gamma}\tau}{D\tau}\right)$ and the hyperbola $\frac{\alpha D}{D-D_0}$, as illustrated in Fig. S1. So that $D = D(G_0\dot{\gamma}\tau, \sigma_c, \alpha, \sqrt{D_0\tau})$ can be computed numerically for any given set of its parameters values, using for instance a straightforward bisection method.

The corresponding mean stress can then be obtained by substituting $D = D(G_0\dot{\gamma}\tau, \sigma_c, \alpha, \sqrt{D_0\tau})$ into (S11)-(S12)-(S13), yielding $\sigma_M = \sigma_M(G_0\dot{\gamma}\tau, \sigma_c, \alpha, \sqrt{D_0\tau})$. They are illustrated by Fig. S2.

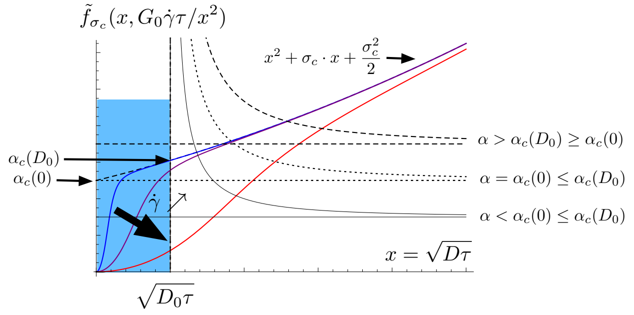


FIG. S1. Schematic plot of the function $\tilde{f}_{\sigma_c}\left(\sqrt{D\tau}, \frac{G_0\dot{\gamma}\tau}{D\tau}\right)$ defined in Eq. (S9), in the presence of a constant external shear rate $\dot{\gamma} \geq 0$. This function in absence of shear, *i.e.* $\tilde{f}_{\sigma_c}\left(\sqrt{D\tau}, 0\right)$, defines the 'critical' coupling $\alpha(0) = \sigma_c^2/2$ of the original HL model, and its counterpart $\alpha(D_0) = \tilde{f}_{\sigma_c}\left(\sqrt{D_0\tau}, 0\right)$ for a finite activity. The steady-state diffusion coefficient is determined geometrically as the $\alpha$-dependent intersection of $\tilde{f}_{\sigma_c}$ with the hyperbola $\alpha x^2/(x^2 - D_0\tau)$, as illustrated for three different values of $\alpha$.

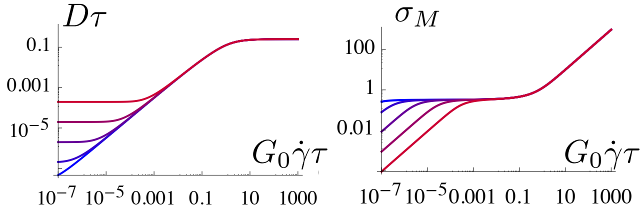


FIG. S2. Steady-state diffusion coefficient and mean stress predicted by the original HL, with a single value for the local yield stress $\sigma_c = 1$, and a fixed coupling $\alpha/\sigma_c^2 = 0.25$. The curves from blue to red correspond to an increasing value for the diffusion threshol $D_0\tau \in \{10^{-8}, 10^{-7}, 10^{-6}, 10^{-5}, 10^{-4}\}$.

### Low-shear-rate perturbative expansions

In the low-shear-rate regime we are interested in, the previous expressions can be simplified within a perturbative expansion. We are focusing exclusively on the regimes at $\alpha < \alpha_c = \sigma_c^2/2$, which displays a Herschel-Bulkley behavior of the flow curve at low shear rates. In addition, we assume that $D_0$ is sufficiently small so that it is relevant only for shear rates below $\dot{\gamma}_*(D_0)$, with $G_0\dot{\gamma}_*\tau \ll 1$. This assumption allows us on the one hand to assume that the usual HL predictions remain valid for $\dot{\gamma} > \dot{\gamma}_*$, and on the other hand to use the same low-shear-rate perturbative expansion at $\dot{\gamma} < \dot{\gamma}_*$ with $D \approx D_0$.

These two regimes are transparent on the diffusion coefficient itself, at $G_0\dot\gamma\tau \ll 1$:

$$\begin{cases} D \approx D_0 & (\text{at } \dot\gamma < \dot\gamma_*) \\ D \approx C_1 G_0\dot\gamma\tau \left[1 + C_2\left(G_0\dot\gamma\tau\right)^{1/2}\right] & (\text{at } \dot\gamma > \dot\gamma_*) \end{cases} \tag{S16}$$

with $C_1$ and $C_2$ given by:

$$\begin{cases} C_1\sigma_c \tanh\left(\frac{\sigma_c}{2C_1}\right) = \alpha \\ C_2 = \sqrt{C_1}\,\frac{\frac{\sigma_c}{2}+C_1\tanh\left(\frac{\sigma_c}{2C_1}\right)-\frac{1}{2}\sigma_c\tanh^2\left(\frac{\sigma_c}{2C_1}\right)}{\frac{\sigma_c^2}{2}-C_1\sigma_c\tanh\left(\frac{\sigma_c}{2C_1}\right)-\frac{1}{2}\sigma_c^2\tanh^2\left(\frac{\sigma_c}{2C_1}\right)} \end{cases} \tag{S17}$$

(see Eqs. (D.10) and (D.11) in Ref. [2]). The crossover $\dot\gamma_*$ can then be simply defined as the intersection of the plateau at $D_0$ and the linear regime as follows:

$$D_0\tau \equiv C_1 G_0 \dot\gamma_*^{(\text{diff})}\tau \Longleftrightarrow \boxed{\dot\gamma_*^{(\text{diff})} = \frac{D_0}{G_0 C_1} \sim D_0} \tag{S18}$$

The different features of the diffusion-coefficient regimes are thus characterized by $\left\{D_0, C_1, C_2, \dot\gamma_*^{(\text{diff})}\right\}$.

The mean stress also has two regimes as a function of the shear rate at $G_0\dot\gamma\tau \ll 1$, consequently to (S16):

$$\begin{cases} \sigma_M \approx \tilde\eta\, G_0\dot\gamma\tau = \eta\,\dot\gamma & (\text{at } \dot\gamma < \dot\gamma_*) \\ \sigma_M \approx \sigma_Y + A\,\left(G_0\dot\gamma\tau\right)^{1/2} = \sigma_y + A_{\text{HB}}\,\dot\gamma^{1/2} & (\text{at } \dot\gamma > \dot\gamma_*) \end{cases} \tag{S19}$$

where we have introduced two different notations for the parameters, depending if they include $G_0\tau$ or not. The explicit expressions for the Herschel-Bulkley behavior at $\dot\gamma > \dot\gamma_*$ are the following:

$$\sigma_Y = C_1\left[\frac{\sigma_c^2/2}{C_1\sigma_c\,\tanh\left(\frac{\sigma_c}{2C_1}\right)} - 1\right] \tag{S20}$$

$$A = \frac{A_{\text{HB}}}{G_0\tau} = \frac{3\sqrt{C_1}}{2}\coth\left(\frac{\sigma_c}{2C_1}\right) + \frac{C_1^{3/2}}{\sigma_c}\left(1 + \frac{\cosh\left(\frac{\sigma_c}{C_1}\right)-1}{1-\frac{C_1}{\sigma_c}\sinh\left(\frac{\sigma_c}{C_1}\right)}\right) \tag{S21}$$

(recalled from Eqs. (19)-(20) of Ref. [2], and detailed furthermore in Appendix E of the same reference). Note that keeping track of the second order correction $C_2$ is necessary in order to obtain the correct expression for $A$. As for the Newtonian behaviour at $\dot\gamma > \dot\gamma_*$, its viscosity is given by:

$$\begin{aligned}\tilde\eta = \frac{\eta}{G_0\tau} &= 1 + \left(\frac{\sigma_c^3}{6\sqrt{D_0\tau}} + \frac{\sigma_c^4}{24 D_0\tau}\right)\frac{1}{\tilde f_{\sigma_c}\left(\sqrt{D_0\tau}, 0\right)} \\ &= 1 + \left(\frac{\sigma_c^3}{6\sqrt{D_0\tau}} + \frac{\sigma_c^4}{24 D_0\tau}\right)\frac{1}{D_0\tau + \sqrt{D_0\tau}\sigma_c + \sigma_c^2/2}\end{aligned} \tag{S22}$$

The crossover $\dot\gamma_*$ can then be defined similarly to (S18) as the intersection of the plateau at the Newtonian regime $\eta\,\dot\gamma$ and the yield-stress plateau $\sigma_Y$ as follows:

$$\eta\dot\gamma_*^{(\text{stress})} \equiv \sigma_Y \Longleftrightarrow \boxed{\dot\gamma_*^{(\text{stress})} = \frac{\sigma_Y}{\eta} = \frac{\sigma_Y}{\tilde\eta G_0\tau}} \tag{S23}$$

The dependence on the threshold $D_0$ is hidden in the viscosity $\tilde\eta$, which can be perturbatively expanded at small $D_0$ as:

$$\tilde\eta \underset{(D_0\to 0)}{\approx} \frac{\sigma_c^2}{12 D_0\tau} + \frac{\sigma_c}{6\sqrt{D_0\tau}} + \frac{1}{2} + \mathcal{O}(\sqrt{D_0\tau}) \tag{S24}$$

So we recover that $\dot\gamma_*^{(\text{stress})} \sim D_0$, as in (S18), although this scaling prefactor differs depending on the criterion used to define the crossover $\dot\gamma_*$, either on the diffusion coefficient or on the mean-stress crossover. The different features of the mean-stress regimes are thus characterized by $\left\{\eta, \sigma_Y, A_{\text{HB}}, \dot\gamma_*^{(\text{stress})}\right\}$.

The equation for $C_1(\sigma_c, \alpha)$ being implicit, the crossover expression can be further simplified only in two specific opposite cases for $\alpha < \alpha_c$, for both our definitions of $\dot\gamma_*(D_0)$. One the one hand:

$$\begin{cases} G_0\dot\gamma_*^{(\text{diff})} \approx D_0\sigma_c/\alpha & (\text{at } \alpha \ll \alpha_c) \\ G_0\dot\gamma_*^{(\text{diff})} \approx D_0\left[24(\alpha_c-\alpha)\right]^{1/2}/\sigma_c^2 & (\text{at } \alpha \lesssim \alpha_c) \end{cases} \tag{S25}$$

and on the other hand:

$$\dot\gamma_*^{(\text{stress})} = \frac{\sigma_Y}{\tilde\eta G_0\tau} = \frac{12\sigma_Y D_0}{\sigma_c^2 G_0} \tag{S26}$$

$$\begin{cases} G_0\dot\gamma_*^{(\text{stress})} \sim D_0\frac{\alpha_c-\alpha}{\sigma_c^3} & (\text{at } \alpha \ll \alpha_c) \\ G_0\dot\gamma_*^{(\text{stress})} \sim D_0\frac{(\alpha_c-\alpha)^{1/2}}{\sigma_c^2} & (\text{at } \alpha \lesssim \alpha_c) \end{cases} \tag{S27}$$

using the perturbative expansions given in Eqs. (D.13), (D.14), (E.3) and (E.4) in Ref. [2].

The different features that we have just discussed corresponds to low-shear-rate expansions of the analytical steady-state solution of the model, and can be summarized as follows:

$$\begin{cases} D = D(G_0\dot\gamma\tau, \sigma_c, \alpha, \sqrt{D_0\tau}) \\ \text{and features to fit are } \left\{D_0, C_1, C_2, \dot\gamma_*^{(\text{diff})}\right\} \end{cases} \tag{S28}$$

$$\begin{cases} \sigma_M = \sigma_M(G_0\dot\gamma\tau, \sigma_c, \alpha, \sqrt{D_0\tau}) \\ \text{and features to fit are } \left\{\eta, \sigma_Y, A_{\text{HB}}, \dot\gamma_*^{(\text{stress})}\right\} \end{cases} \tag{S29}$$

The shear-rate dependence of the stress diffusion coefficient $D(\dot\gamma)$ and the corresponding flow curve $\sigma_M(\dot\gamma)$ are shown in Fig. S2.

We mention at last that the validity of these mean-field predictions is discussed, at a qualitative level, in the broader framework of the athermal local-yield stress (ALYS) models at fixed shear rate, in Ref. [3]. We know in particular that the Herschel-Bulkley behaviour

of exponent 1/2 is robust with respect to a partial relaxation of stress, although the specific predictions for $\{\sigma_Y, A_{\rm HB} = A\,G_0\tau\}$ will depend on the *a priori* distribution $\rho(\sigma_c)$, and on the specific partial relaxation of the local stress after a plastic event. The prediction for a Newtonian regime $\sigma_M \approx \eta(D_0)\,\dot\gamma$ at very low shear rates is similarly robust to the addition of disorder and partial relaxation. This means in particular that the collapse of the flow curves using that $\dot\gamma_* \sim D_0$ should remain valid.

## FURTHER MODEL DETAILS AND GPU-PARALLEL MOLECULAR DYNAMICS IMPLEMENTATION

A remarkable amount of information about collective behavior at tissue level can be obtained from effective models where cells are treated as soft elastic objects. Particle-based tissue models have been successfully applied to a wide range of systems, for a complete review see Drasdo *et al.* [5] and references therein. Here we follow a similar approach and consider a model where the cells are represented by soft spheres of radius $b_i$. Therefore, the tissue consists in a collection of $N$ such spheres with radii $b_i$ interacting via a soft elastic potential given by,

$$V_{ij} = \begin{cases} \frac{1}{2}kb_{ij}^2\left[\left(\frac{r_{ij}}{b_{ij}}-1\right)^2-\epsilon^2\right] & \text{if } \frac{r_{ij}}{b_{ij}}-1\le\epsilon \\ -\frac{1}{2}kb_{ij}^2\left(\frac{r_{ij}}{b_{ij}}-1-2\epsilon\right)^2 & \text{if } \epsilon<\frac{r_{ij}}{b_{ij}}-1\le 2\epsilon, \end{cases} \tag{S30}$$

where $k$ is the stiffness constant, $b_{ij} = b_i + b_j$ is the sum of the particle radii, and $(b_{ij}\epsilon)$ is the adhesive force strength. The corresponding force of Eq. (S30) is given by Eq. (1) in the main text (see Fig. S3).

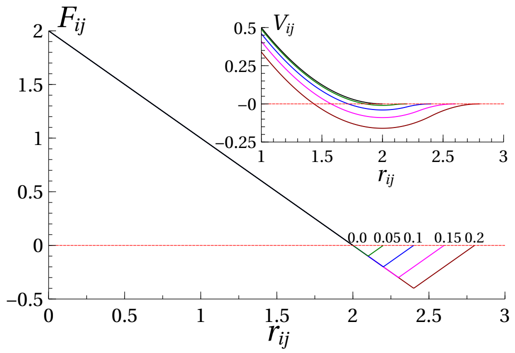


FIG. S3. The elastic force [Eq. (1) in the main text] for $k = 1$ and different values of the adhesive force strength $\epsilon$, as indicated in the figure. (*Inset*) Interparticle potential $V_{ij}$, given in Eq. (S30).

Neglecting inertia effects we model the dynamics of the cell positions $\mathbf{r}_i(t)$ as fully overdamped [6]

$$\partial_t \mathbf{r}_i(t) = \mu \mathbf{F}_i, \tag{S31}$$

where $\mu$ is the inverse friction coefficient and $\mathbf{F}_i = \sum_{j\neq i}\mathbf{F}_{ij}$ is the total force acting on particle $i$ exerted by its neighbours. We integrate the equation of motion (S31) using a C++ GPU-parallel Molecular Dynamics code described in the following section.

### GPU-Parallel Implementation

It is well known that Molecular Dynamics (MD) simulation is a highly parallelizable numerical method. Following the spirit of MD packages such as LAMMPS, AMBER, GROMACS, etc., we have built our own parallel MD code on GPU (NVIDIA CUDA). In contrast to LAMMPS, for example, our in-house code is specifically designed to introduce different sources of activity into the system (cell division, cell death and self-propulsion velocities). The general workflow of the code is shown in algorithm 1. All our routines are fully implemented on the GPU, so that there are no transfers between DEVICE-HOST during the MD execution. The only routines executed by the host (colored in blue) are those required by the user in order to save data. It is worth mentioning that these operations require data transfer between the DEVICE and the HOST, see the red colored text.

Our CUDA kernels are moderately optimized, trying to keep aligned and coalesced memory access, and avoiding threads divergence and atomic functions. Further optimizations are still possible, but there are diminishing returns since at some point they will obfuscate the code for a negligible speedup. As defensive programming techniques we use assertions, and each routine is independently tested before implementation. We do not use heavy database implementations and/or post-processing packages: in most cases the output of our simulation is already the final result. Finally, we used external imaging routines for visualization, testing and presentation purposes.

**Algorithm 1:** Typical Simulation Scheme

**(0) Give atoms initial positions and velocities;**
**for** *Simulation time* **do**
**(1) Predict next atom positions:**
(a) Get Forces;
(b) Move Atoms and Update Velocities;
(c) Apply Boundary Conditions;
(c*) Deform the box during force-shear simulations;
**(2) Cell Functions:**
(a) Cell death;
(b) Cell division;
**(3) Build neighbours:**
**if** *(2) or atoms move too far* **then**
(a) Build the linked-list;
(b) Using (a) build the neighbour list of each atom;
**(4) Analysis:**
**if** *Simulation time* **then**
(a) Standard properties: pressure, density, etc.;
(b) Transport properties: Mean square displacement etc.;
(c) Transfer (a) and (b) to the host (CPU);
(d) Save (a) (b);
**(5) Save Configurations:**
**if** *Simulation time* **then**
(a) Transfer atom properties to the host (CPU);
(b) Save (a);

* daniel-alejandro.matoz-fernandez@univ-grenoble-alpes.fr

† elisabeth.agoritsas@lpt.ens.fr

[1] P. Hébraud and F. Lequeux, Phys. Rev. Lett. **81**, 2934 (1998).
[2] E. Agoritsas, E. Bertin, K. Martens, and J.-L. Barrat, Eur. Phys. J. E **38**, 71 (2015).
[3] E. Agoritsas and K. Martens, "Nontrivial rheological exponents in sheared yield stress fluids," arXiv:1602.03484 [cond-mat.soft] (2016).
[4] J. A. Dijksman, G. H. Wortel, L. T. H. van Dellen, O. Dauchot, and M. van Hecke, Phys. Rev. Lett. **107**, 108303 (2011).
[5] D. Drasdo, S. Hoehme, and M. Block, J. Stat. Phys. **128**, 287 (2007).
[6] S. Henkes, Y. Fily, and M. C. Marchetti, Phys. Rev. E **84**, 040301 (2011).
